# Supplementary material for: Think Right, Not More: Test-Time Scaling for Numerical Claim Verification
Source: arXiv:2509.22101 source file (2025-09-26)
Supplement: Supplementary file 1 [file appendix_re_rank_results.tex]

\begin{table}[!t]
    \centering
    \small
    \setlength{\tabcolsep}{2.0pt}
    \begin{tabular}{lccc}
    \toprule
     \textbf{Method}& \multicolumn{1}{c}{MQA}& \multicolumn{1}{c}{\wqa{}}\\

     % & cover-EM & cover-EM& EM& EM&EM \\
     \midrule
          \colorg \textbf{Methods (w/o query understanding)} & \colorg& \colorg& \colorg\\
     
     \zfshot{} \cite{kojima2023large}  & 8.62 & 30.42 \\
%          \COT{} + re-rank &23.64& 44.92 \\
     \COT{} \cite{wei2023chainofthought} &15.02& 32.83 \\

               \COT{} +PRF \cite{ance_prf} & 16.69 & 35.55 \\
$\name{}_R$ (ours) & 21.32 & 40.96 \\
$\name{}$ (ours) & & \\

    \hline
              \colorg \textbf{Methods (w/ query understanding)} & \colorg& \colorg& \colorg\\
    %\self{} \cite{self_ask} & 15.00& 32.92 \\

 %   ReAct \cite{yao2023react} & 9.03 & 28.67  \\
   %     ReAct + re-rank \cite{yao2023react} & 19.65 & 42.75  \\

    Self-RAG \cite{asai2024selfrag} & 17.80 & 35.25 \\
    ReAct \cite{yao2023react} & 21.41 & 43.25  \\

    DecomP \cite{khot2023decomposed} & 21.01 & 44.08 \\
   % DsPy \cite{khattab2023dspycompilingdeclarativelanguage} & & \\
   % SearChain \cite{xu2024searchinthechaininteractivelyenhancinglarge} & 17.07 & 30.92 \\
   % SearChain + re-rank & 19.72& 41.75 \\ 

        SearChain \cite{xu2024searchinthechaininteractivelyenhancinglarge} & 21.72& 44.42  \\ 
            \COT{} +PRF \cite{ance_prf} &  & 44.58 \\

            \self{} \cite{self_ask} & 24.84& 45.75 \\

%    \self{} + re-rank & 24.44& 44.08 \\

  %  \self{} + re-rank + MER & 24.84& 45.75 \\

   %     \self{} + re-retrieval & 24.84& 45.75 \\
    %    \self{} + re-retrieval + MER & 26.99& 47.75 \\
        \hline
                 \colorg \textbf{NAR (w/ query understanding) (ours)}& \colorg& \colorg& \colorg\\

        $\name{}_{R}$ & 28.11 & 47.67\\  
       %   Adaptive Retrieval + MER & 31.79 & 52.5\\
        \name{} & \textbf{32.75} $\dagger$& \textbf{54.83}$\dagger$ \\
        \hline  \hline
                 \colorg \textbf{Golden Evidence }& \colorg& \colorg& \colorg\\   
                                  \colorg \textbf{(Ideal Upper Bound)}& \colorg& \colorg& \colorg\\
                 \COT{} & \colorit 44.28     &  \colorit  65.55  \\

     \bottomrule
    \end{tabular}
    \caption{Results across datasets. The model used for \name{} and other approaches is gpt-3.5-turbo unless otherwise specified.$\dagger$ indicates statistical significance over \self{} at 0.1 level.}
    \label{tab:main_result}
\end{table}
